# Supplementary material for: Observation of Interaction of Spin and Intrinsic Orbital Angular Momentum of Light
Source: arXiv:1607.06192 ancillary file (2017-02-21)
Supplement: Supplementary file 1 [file ISOI_Supplement_arXiv_v3.pdf]

# Observation of Interaction of Spin and Intrinsic Orbital Angular Momentum of Light: Supplementary Material

Dashiell L. P. Vitullo,[1] Cody C. Leary,[2] Patrick Gregg,[3] Roger A. Smith,[1]
Dileep V. Reddy,[1] Siddharth Ramachandran,[3] and Michael G. Raymer[1]

[1] *Department of Physics and Oregon Center for Optical, Molecular, & Quantum Science, University of Oregon, Eugene, OR 97403, USA**
[2] *Department of Physics, College of Wooster, Wooster, OH 44691, USA*
[3] *Department of Electrical & Computer Engineering, Boston University, Boston, MA 02215, USA*

## PREPARATION AND CHARACTERIZATION OF INPUT AND OUTPUT BEAMS

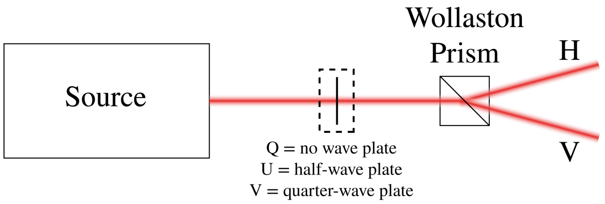


FIG. S1. Polarimeter setup. Power is measured for both outputs from the Wollaston prism, labeled H and V for horizontal or vertical with respect to the prism basis. The dashed box indicates three possible configurations and which parameter is measured when the corresponding wave plate is present.

We measure polarization content of our beams with a polarimeter consisting of a Wollaston prism, achromatic half- and quarter-wave plates, and power meters, as shown in Fig. S1. Polarization measurements for a beam with electric field $E$ are found by splitting the input beam into two orthogonally polarized beams in three bases [1]. The normalized Stokes parameters are

$$I = \langle|E_H|^2\rangle + \langle|E_V|^2\rangle \tag{S1}$$

$$Q = \frac{\langle|E_H|^2\rangle - \langle|E_V|^2\rangle}{\langle|E_H|^2\rangle + \langle|E_V|^2\rangle} \tag{S2}$$

$$U = \frac{\langle|E_D|^2\rangle - \langle|E_A|^2\rangle}{\langle|E_D|^2\rangle + \langle|E_A|^2\rangle} \tag{S3}$$

$$V = \frac{\langle|E_L|^2\rangle - \langle|E_R|^2\rangle}{\langle|E_L|^2\rangle + \langle|E_R|^2\rangle}, \tag{S4}$$

where $H/V$ indicate horizontal/vertical, $D/A$ indicate diagonal/anti-diagonal, $L/R$ indicate left-/right-circular polarization, and $\langle\,\rangle$ indicates time averaging and integration over the whole transverse extent of the beam. The coordinates on the Poincaré sphere are

$$\mathrm{DOP} = \sqrt{Q^2 + U^2 + V^2} \tag{S5}$$

$$\theta = \tan^{-1}\left(\sqrt{Q^2 + U^2}/V\right) \tag{S6}$$

$$\phi = \tan^{-1}(U/Q), \tag{S7}$$

as illustrated in Fig. S2. The degree of polarization (DOP) is the length of the polarization vector, has a value between 0 and 1, and indicates the degree of spatial and temporal uniformity of the polarization. $\theta$ is the polar angle that describes "how circular" the polarization is, has a value between 0°, denoted left-circularly polarized (LCP, $\sigma = +1$) and 180°, denoted right-circularly polarized (RCP, $\sigma = -1$) with linear polarization lying on the "equator" defined by $\theta = 90°$. The azimuthal angle $\phi$ gives the orientation of the semi-major axis of the polarization ellipse, and has range $-180° < \phi < 180°$. Note that horizontal and vertical polarization are 180° away from each other on the Poincaré sphere, as 2 Poincaré degrees = 1 degree in configuration space.

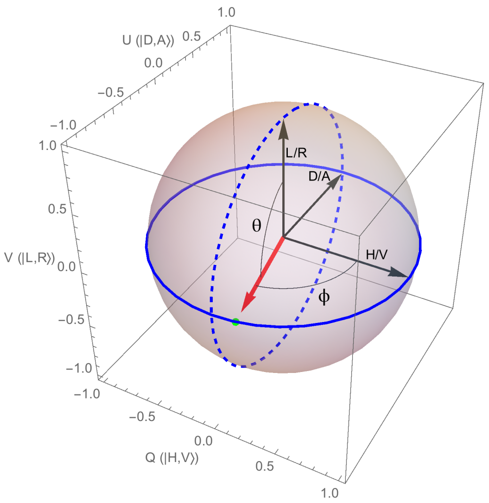


FIG. S2. The polarization Poincaré sphere. A polarization state vector is shown as the red vector. The state with DOP=1 would intersect the sphere at the green point.

Together with Fig. 5 from the main manuscript, Fig. S3(a) and Fig. S3(b) give full polarization information, and display $\theta$ *vs.* fiber length $L$ and DOP *vs.* $L$, respectively.

The linearly polarized inputs stay close to linearly polarized at the output with $\theta \approx 90°$ while the circularly polarized inputs oscillate between well circularly polarized and elliptical polarization. The DOP remains consistently high for the fundamental, but varies between low

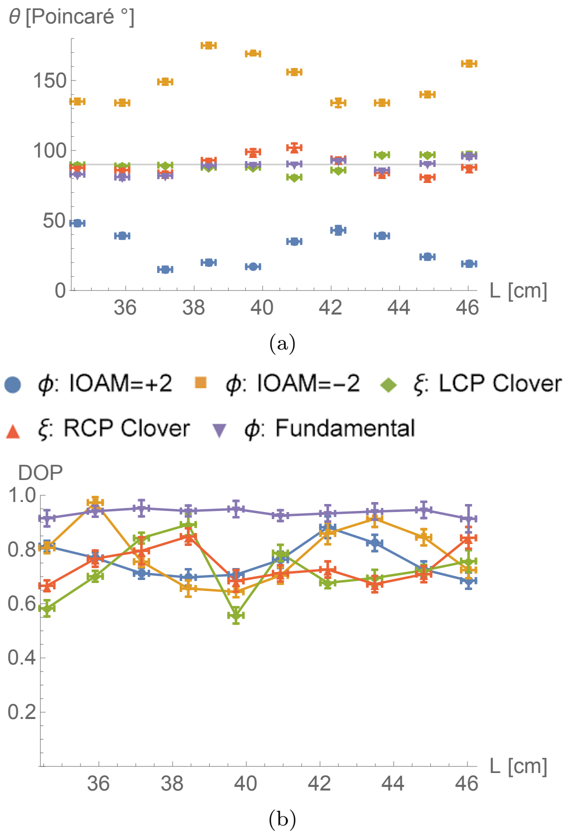


FIG. S3. (a) Polar polarization angle $\theta$ for all 5 input settings. Grey line at 90 Poincaré ° is an eye-guide for linear polarization. The legend association between color, shape, and input profile holds for all data plots. (b) Degree of polarization vs. $L$. Colored lines serve as eye-guides.

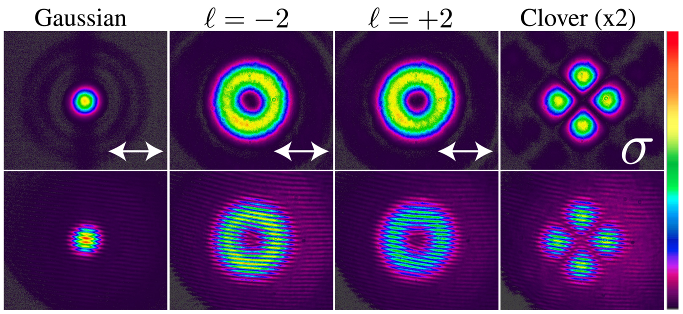


FIG. S4. Input intensity profiles (top row) and interferograms (bottom row). Arrowed lines indicate the linear polarization axis, while $\sigma$ indicates circular polarization. Zooming in on the interferograms, the difference between the number of fringes on the right and left sides of the beam indicate the IOAM charge.

values within the range of roughly 0.6 to 0.9 for $|\ell| = 2$ modes. This behavior is consistent with intermodal coupling, discussed in the next section.

The holograms used on the reflective phase-only Holoeye HEO1080P spatial light modulator (SLM) to generate desired spatial patterns at the fiber input are shown in Fig. S6. Holograms were designed following the approach of [2] using Mathematica code modified from code shared by the Glasgow group [3]. To create the desired complex-valued transverse field distribution $f(x,y)$, normalized so the range of $|f(x,y)|^2 \in [0,1]$, from an input collimated Gaussian beam, the hologram $H(x,y)$ is

$$H(x,y) = \text{SLM}\left[\frac{|f(x,y)|^2}{2}\left(\frac{P(x,y)}{\pi} - 1\right) + \frac{1}{2}\right] \quad \text{(S8)}$$

$$P(x,y) = \text{Mod}\left[\mathscr{P}(x) + \mathscr{L}(x,y) + \text{Arg}\left(f(x,y)\right)\right] \quad \text{(S9)}$$

where $P(x,y)$ is the combined phase profile, the modulus function, Mod, gives the remainder of it's argument divided by $2\pi$, the prism function $\mathscr{P}(x) = \frac{2\pi}{\lambda_x}x$, the lens function $\mathscr{L}(x) = \frac{-\pi}{\lambda f_H}(x^2 + y^2)$, the argument function Arg gives the phase of it's argument, and the SLM function takes input in the range $[0,1]$ and maps it to discretized SLM pixel settings. The range of possible pixel settings is lightly restricted to an integer in $[0,245]$ from the designed maximum setting of 255 so the maximum phase shift at a pixel is closer to $2\pi$ at our design wavelength, $\lambda = 800$ nm. The $\lambda_x$ parameter controls the slope of $\mathscr{P}$, and thus the angular separation of the diffractions orders from the hologram, which allows us to isolate our desired first-order diffracted beam. $f_H$ is the focal length of the effective spherical lens used to control the focal properties of the output beam. We use a Laguerre-Gauss mode basis for $f(x,y)$. Interfering the input beams with a reference wave that has a flat phase distribution creates interferograms, shown in Fig. S4, which reveal the input beam's phase structure.

Fig. S7 contains all output profiles and interferograms. The red crosshairs on clover profiles track the orientation angle $\xi$. The crosshairs are added in image editing software and $\xi$ is manually assessed by rotating them into alignment with the nodal lines. The $\pm 2°$ uncertainty of this method is much smaller than the $\sim 15°$ clover rotation between $L$ values. The periodicity of $\phi$ and $\xi$ makes for a sawtooth profile in the output measurements where $\xi \in [0, 90°)$ and $\phi \in [0, 180°)$. Adding appropriate integer multiples of 90° to $\xi$ values and 180° to $\phi$ values "linearizes" the sawtooth to facilitate extracting the rotation rate with a linear least-squares fit. The output profiles show distortion that indicates mode coupling. Profile size differences are due to small differences in the distance between the output objective lens system and the fiber output that do not affect polarization or orientation.

## MODE COUPLING

In multimode fiber, unavoidable imperfections in geometry and strain couple energy between modes [4]. This coupling depends on defect symmetry and separation between modal propagation constants $\beta$ [5]. Modes with small differences between their $\beta$ values couple most readily.

We performed numerical investigation of propagation with coupling that illuminates expected behavior, but does not give a fit mapping the imperfections underlying the observed curves. The dispersion-tailored fiber used in our experiment is designed to have $|\ell| = 2$ modes isolated from other modes, so we expect coupling to be dominantly between $|\ell| = 2$ modes. This is consistent with the output spatial profile data in Fig. S7, where the number of nodal lines and phase singularities is preserved. The $\ell = \pm 2$ inputs give output profiles with intensity depressions that look similar to nodal lines, as modes with opposite IOAM are populated, but with a smaller excitation amplitude than the input IOAM profile. Similarly, oscillation in Figs. S3(a) and S3(b) are consistent with intermodal coupling. The magnitude of the $\phi$ and DOP oscillations for $|\ell| = 2$ modes, as well as the linearity of both $\phi$ and $\xi$ *vs.* $L$ in Fig. 5 bounds the coupling strength and error in the $\delta\beta$ measurement, and the magnitudes observed are consistent with error of the same magnitude as our calculated uncertainty. Strong coupling causes $\phi(L)$ and $\xi(L)$ to depart from linear behavior, and while small oscillations are visible in Fig. 5, the goodness of linear fits as measured by $R^2$ coefficients is $> 0.987$ for all $|\ell| = 2$ settings, indicating good agreement with linear behavior.

## FIBER DETAILS AND EXACT MODE SIMULATION

The perturbative approach of Eqn. 5 in the main manuscript provides insight into the physical causes of spin-IOAM interaction, and predicts correctly the behaviors observed in the experiment. The SOI physics is obscured in the exact mode description, but it should provide the most accurate predictions for the slopes of the rotation-versus-length curves of Fig. 5. Thus, numerical solutions for the propagation constants of the exact vector modes of the fiber are considered here.

An Interfiber Analysis IFA-100 fiber profiler was used to obtain the radial index profile of the fiber (see Fig. S5) and checked to be consistent along the fiber. The measured index profile is input to a finite difference algorithm that solves the coupled differential equations (from Maxwells equations) describing the modal field components. The algorithm finds the characteristic $\beta$ values, (or equivalently the effective indices $n_{\text{eff}} = \beta/k$ where $k$ is the vacuum wavenumber), for a set of fiber modes that

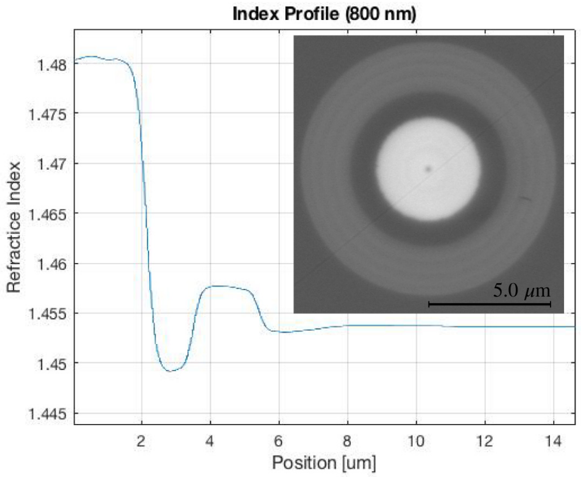


FIG. S5. Refractive index profile of the dispersion tailored fiber used in our experiment for 800 nm light. The inset shows a scanning electron microscope (SEM) image of dispersion-tailored fiber core structure.

includes the modes of interest. The exact fiber modes corresponding to our $|\ell| = 2$ modes of interest are the two polarizations of $HE_{3,1}$ (with parallel spin-IOAM orientation) and the two polarizations of $EH_{1,1}$ (with anti-parallel spin-IOAM orientation) [6]. The group index crossing between $EH_{1,1}$ and $HE_{3,1}$ modes, referred to as the turn-around point (TAP), is measured to occur at 848.0 nm in our experimental fiber, and agreement of the measured and predicted TAP is used to validate the simulation. The simulated difference in the effective index experienced by $HE_{3,1}$ modes and that experienced by $EH_{1,1}$ modes at $\lambda = 800$ nm is $\Delta n_{\text{eff}} = 1.16 \times 10^{-4}$. For $|\ell| > 1$ modes, the splitting $\delta\beta$ is related to $\Delta n_{\text{eff}}$ by

$$\Delta n_{\text{eff}} = \frac{\delta\beta\,\lambda}{\pi}. \tag{S10}$$

The average splitting value from the best-fit lines of Fig. 5, including the factors of $|\ell| = 2$ to get $\delta\beta$ from the spatial profile rotation, is $(22.1 \pm 0.7)^\circ/\text{cm}$. The slope uncertainties may be correlated, so the error bound of 0.7 is the average of the fit errors, not the combination in quadrature [7]. This splitting corresponds to an experimentally measured effective index difference of $\Delta n_{\text{eff}} = 9.82 \times 10^{-6}$. The simulated $\Delta n_{\text{eff}}$ is larger than the experimentally measured value by a factor of 11.8.

This disagreement is not due to aliasing. The fiber segments removed from the output end of the fiber with a Fujikura high-precision CT-30 cleaver are of slightly different lengths, and the length of the segment (precisely measured with calipers) does not correspond to the deviation in rotation angle expected if the underlying rotation rate were faster than we report. Experimental rotation rates are consistently smaller than predicted by simulation at multiple wavelengths. The symmetry of the mag-

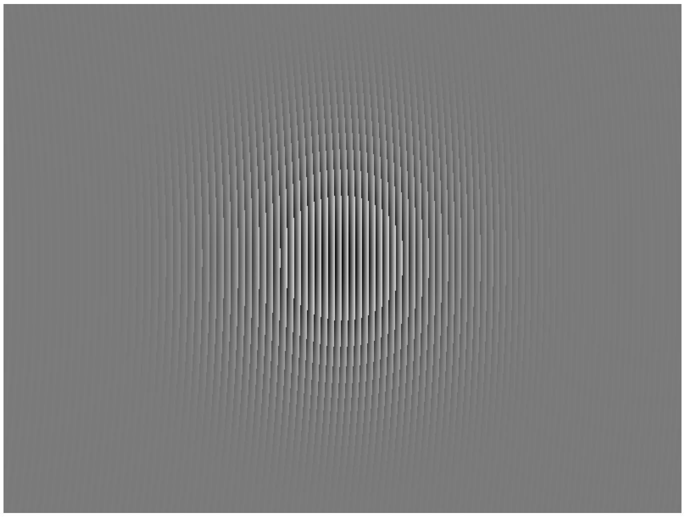

(a)

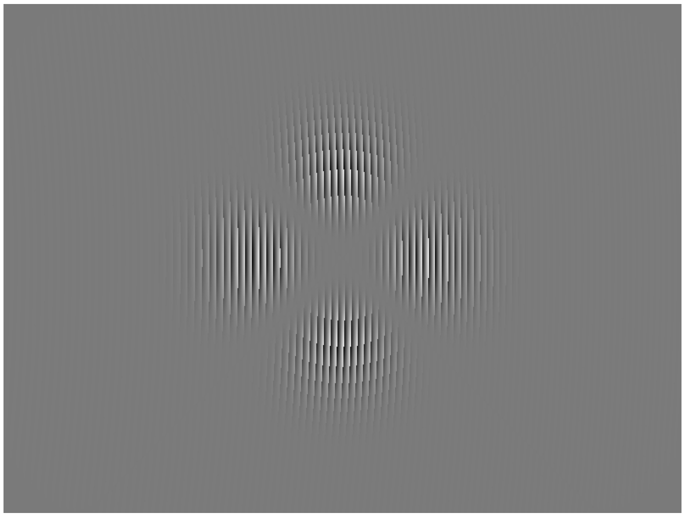

(b)

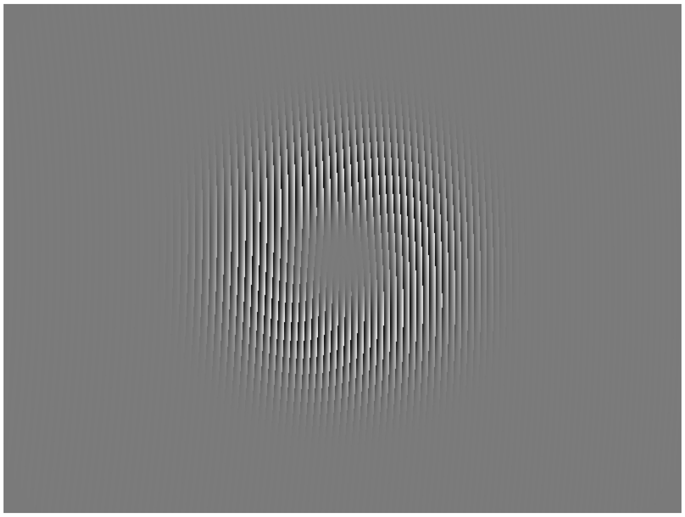

(c)

FIG. S6. Holograms used to generate (a) fundamental, (b) clover, and (c) $\ell = -2$ donut patterns. The fast linear phase ramp acts as a prism and the radial variation acts as a lens to achieve desired direction and focal properties in the generated beams.

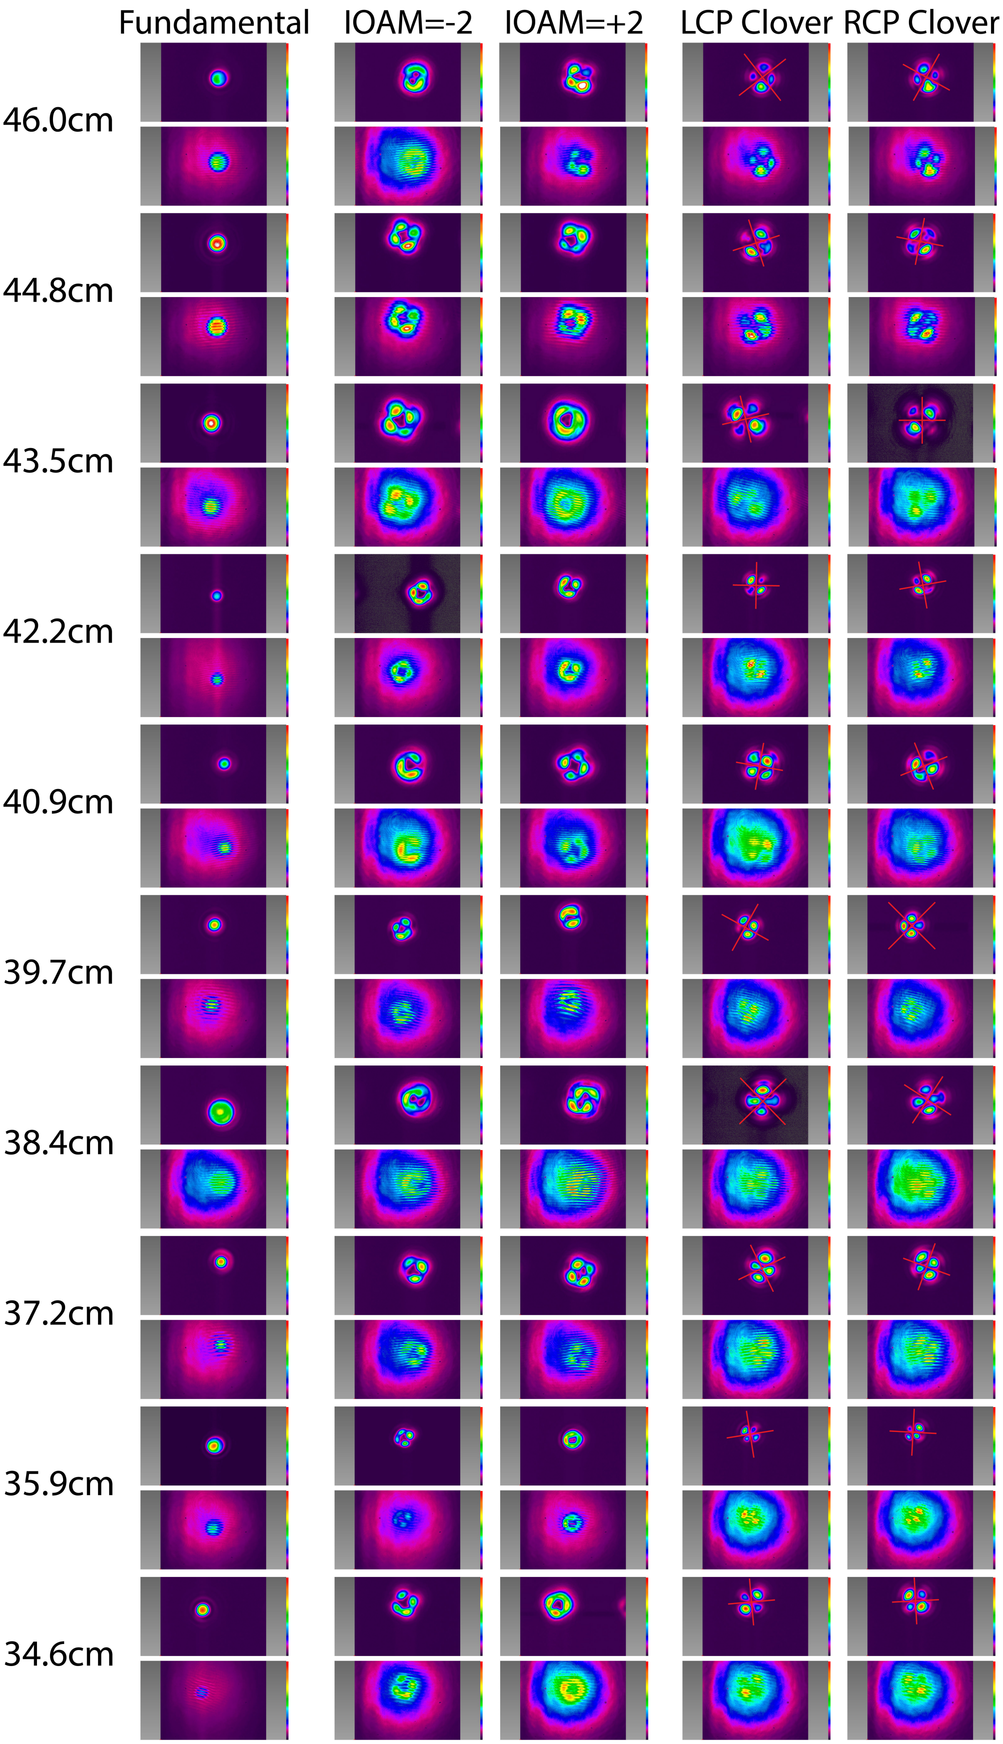


FIG. S7. For each fiber length, sorted vertically, output profiles in the top row above and interferograms in the bottom row. The highest intensity is white, which indicates saturated intensity. Crosshairs used in clover output angle measurement ($\xi$) are included. High resolution should allow for substantial zoom.

nitude of the rotation rates for both control variable signs indicates the absence of additional splittings (*e.g.* optical activity) that offset $\beta$ differently for different values of $\sigma$ or $\mu$. Experimental observation of orbit-controlled spin rotations and spin-controlled orbital rotations, with rotation rates related by the proper factor of 2, as well as the negligible rotation of the polarization of the fundamental, all indicate clean observation of spin-IOAM interaction. The origin of the disagreement between the simulated splitting, validated with proper TAP prediction, and the experimental observed splitting is the subject of ongoing research.

## PATH-DEPENDENT ROTATIONS

The expected geometric phase accumulated by a quantum particle with spin while traversing a 3D path is

$$\Phi_G = -(s\sigma + \ell)\Omega, \tag{S11}$$

where $s$ is the spin magnitude (which is 1 for photons and 1/2 for electrons), $\sigma = \pm 1$ is the particle helicity, $\ell$ is the IOAM quantum number, and $\Omega$ is the solid angle subtended by the path of the centroid of a wave packet in momentum space. A typical means to define such a path is to coil a fiber into a helix [8–10]. In order to get a sense of the magnitude of the effects of taking a three-dimensional path through space, which results in spin-EOAM (geometric phase) rotations, we undertook a qualitative investigation before starting the experiment. A clover profile was coupled through the straight fiber, and then the fiber output was moved closer to the input and the path between the endpoints controlled by hand. Twisting the orientation of a loop of fiber, located more than 30 cm from the fiber input, around the experimenter's hand produced obvious rotations in the output clover profile, but as expected, this required substantial deviations from a straight path, and did not exceed rotations of order 10 degrees. Allowing the fiber to sag under gravity did not produce visible rotations, as is expected for any path that stays in a 2D plane.

The fiber input and output were aligned with the laser before the mode coupling procedure was undertaken, and the output mount was moved along a straightedge that is mounted to the table and aligned to keep the path straight during the cutback experiment. Any deviations from a straight path produced rotations of magnitude much smaller than observed between fiber lengths, and do not explain the approximately 200° total rotation observed in the cutback experiment.

* raymer@uoregon.edu


[1] W. H. McMaster, Am. J. Phys. **22**, 351 (1954).

[2] J. Leach, M. R. Dennis, J. Courtial, and M. J. Padgett, New J. Phys. **7**, 1 (2005).

[3] T. W. Clark, R. F. Offer, S. Franke-Arnold, A. S. Arnold, and N. Radwell, Opt. Express **24**, 6249 (2016).

[4] S. Ramachandran and P. Kristensen, Nanophotonics **2**, 455 (2013).

[5] P. Gregg, P. Kristensen, and S. Ramachandran, Optica **2**, 267 (2015), arXiv:1412.1397.

[6] A. W. Snyder and J. D. Love, *Optical Waveguide Theory* (Chapman and Hall, New York, 1983).

[7] J. R. Taylor, *An Introduction to Error Analysis*, 2nd ed. (University Science Books, Sausalito, CA, 1982).

[8] C. C. Leary, M. G. Raymer, and S. J. van Enk, Phys. Rev. A **80**, 061804 (2009).

[9] A. Tomita and R. Y. Chiao, Phys. Rev. Lett. **57**, 937 (1986).

[10] I. Bialynicki-Birula and Z. Bialynicka-Birula, Phys. Rev. D **35**, 2383 (1987).
